# Supplementary material for: Contego: An Adaptive Framework for Integrating Security Tasks in Real-Time Systems
Source: arXiv:1705.00138 source file (2017-05-23)
Supplement: Supplementary file 1 [file appendix.tex]

\documentclass[../rt_server_main.tex]{subfiles}

 \begin{document}

%\section*{Appendix}

%\newpage
\appendix

% \section{Real-time and Security Tasks \\ used in the Experiments} \label{appsec:task_param}

% \subfile{Sections/rt_task_table}
% \subfile{Sections/se_task_table}

\section{Solution to the Optimization Problems} \label{appsec:gp}

\subfile{Sections/gp_overview}

 \end{document}
